# Supplementary material for: RiemannONets: Interpretable Neural Operators for Riemann Problems
Source: arXiv:2401.08886 source file (2024-04-16)
Supplement: Supplementary file 1 [file appendix.tex]

\section*{Appendix}
